# Supplementary material for: Aligning Extraction and Generation for Robust Retrieval-Augmented Generation
Source: arXiv:2503.04789 source file (2025-11-17)
Supplement: Supplementary file 1 [file 6-supp.tex]

\section*{Supplementary Material}

We include detailed descriptions of experimental setup, hyperparameter configurations, datasets.

\section{Training Configuration}
\label{sec:exp_setup}

For preference alignment, we explore four approaches. The specifics of each configuration are outlined below.

\paragraph{Supervised Fine-tuning (SFT)} We fine-tune the model using QLoRA \cite{dettmers2024qlora} and DeepSpeed (Stage-2) \cite{rasley2020deepspeed} on a cluster of four NVIDIA H100 GPUs. The fine-tuning process runs for 9,000 steps with AdamW as the optimizer, employing a batch size of 32, an initial learning rate of 5e-4, and a weight decay of 0.05.
To maintain consistency across different SFT approaches, we use the same training setup for all SFT variants (SFT-\{Best, Acc, LLMEval, ROUGE, BERT\}) regardless of how the best output completion is determined. The primary distinction in SFT lies in how the model is conditioned: it is trained on the input paired with a single reference output, which is chosen based on a specific selection criterion. For example, this reference may correspond to the Ext2Gen output that achieves the highest average score across four evaluation metrics.

\paragraph{Direct Preference Optimization (DPO)} We fine-tune the model using DPO \cite{rafailov2024direct}. Since the model has already undergone instruction tuning, we directly apply DPO for further optimization. Similar to SFT, we utilize QLoRA and DeepSpeed (Stage-2) to train the model on a four NVIDIA H100 GPU setup. The training process spans 9,000 steps, employing AdamW as the optimizer with a batch size of 32, an initial learning rate of 5e-6, and a weight decay of 0.05.

\paragraph{Others} 
For further analysis on a different backbone, Qwen2.5-3b-instruct, in Table \ref{table:exp1-qwen} and comparisons with other optimization techniques, including KTO and SimPO (in Table \ref{table:comparision_kto_simpo}), we follow the exact same setup as DPO.

\section{Data Statistics}
\label{sec:stat}

Table \ref{table:source_datasets} presents the statistics of the \algname{} training dataset (150K feedback for \texttt{Ext2Gen-R2}). To ensure dataset balance across types, we processed the data so that each source contains the same number of feedback samples. For HotPotQA and MS-MARCO using original QA and chunks, the input prompt length is shorter than that of the three other datasets, i.e., CNN/DM, PubMed, and GovReport, we created for a more challenging scenario.

\begin{table}[h]
\begin{center}
\scriptsize
\begin{tabular}{|L{1.2cm}|X{1.0cm}|X{1.0cm}|X{1.0cm}|X{1.0cm}|X{1.0cm}|}
\toprule
Dataset &
Domain &
\makecell{\# of \\Instances} &
\makecell{Prompt \\ \!\!\!\!Word count\!\!\!\! } &
\makecell{Chosen\\  Answer \\ \!\!\!\!Word count\!\!\!\!} &
\makecell{Rejected\\ Answer \\ \!\!\!\!Word count\!\!\!\!} \\ \midrule
HotPotQA & Wiki & 25,000 & 746 & 74 & 76 \\
MS-MARCO (Desc.) & Web Search & 25,000 & 1,105 & 130 & 138 \\
MS-MARCO (Non-desc.) & Web Search & 25,000 & 1,097 & 157 & 166 \\
CNN/DM & News & 25,000 & 3,090 & 133 & 177 \\
PubMed & Medical & 25,000 & 3,875 & 151 & 157 \\
GovReport & Report & 25,000 & 3,563 & 177 & 184 \\ \bottomrule
\end{tabular}
\vspace{0.2cm}
\caption{Statistics of the \algname{} training set. We prsent the number of pairwise feedback from each source data and the average number of words in its prompt, chosen, and rejected answers.}
\label{table:source_datasets}
\end{center}
\vspace{-0.7cm}
\end{table}
